# Supplementary material for: Poles of degenerate Eisenstein series and Siegel-Weil identities for exceptional split groups
Source: arXiv:2205.06288 source file (2022-05-12)
Supplement: Supplementary file 1 [file E6.tex]

\begin{landscape} 
  \begin{table} 
 \caption{$E_{6}$ Parabolic 1 dom weight} 
 \begin{tabular}{ccc}
Range & dom weight  & w \\
$ 0 \le s < \frac{1}{12} $ & $ \left[1, 1, 12 s, -12 s + 1, 12 s, -12 s + 1\right] $ & $ w_{6}w_{4}w_{5}w_{2}w_{4}w_{3}w_{1} $ \\
$ \frac{1}{12} \le s < \frac{1}{6} $ & $ \left[1, -12 s + 2, 1, 12 s - 1, -12 s + 2, 12 s - 1\right] $ & $ w_{5}w_{2}w_{4}w_{3}w_{1} $ \\
$ \frac{1}{6} \le s < \frac{1}{4} $ & $ \left[1, 12 s - 2, 1, -12 s + 3, 12 s - 2, 1\right] $ & $ w_{4}w_{3}w_{1} $ \\
$ \frac{1}{4} \le s < \frac{1}{3} $ & $ \left[1, 1, -12 s + 4, 12 s - 3, 1, 1\right] $ & $ w_{3}w_{1} $ \\
$ \frac{1}{3} \le s < \frac{5}{12} $ & $ \left[-12 s + 5, 1, 12 s - 4, 1, 1, 1\right] $ & $ w_{1} $ \\
$ \frac{5}{12} \le s \le \frac{1}{2} $ & $ \left[12 s - 5, 1, 1, 1, 1, 1\right] $ & $ 1 $ \\
\end{tabular} \end{table} 
  \end{landscape} \begin{landscape} 
  \begin{table} 
 \caption{$ E _{ 6 }$ Parabolic 2 dom weight} 
 \begin{tabular}{ccc}
Range & dom weight  & w \\
$ 0 \le s < \frac{1}{22} $ & $ \left[1, -11 s + \frac{1}{2}, -11 s + \frac{1}{2}, 22 s, -11 s + \frac{1}{2}, 1\right] $ & $ w_{5}w_{6}w_{3}w_{2}w_{4}w_{5}w_{1}w_{3}w_{4}w_{2} $ \\
$ \frac{1}{22} \le s < \frac{3}{22} $ & $ \left[-11 s + \frac{3}{2}, 11 s - \frac{1}{2}, 11 s - \frac{1}{2}, -11 s + \frac{3}{2}, 11 s - \frac{1}{2}, -11 s + \frac{3}{2}\right] $ & $ w_{6}w_{4}w_{5}w_{1}w_{3}w_{4}w_{2} $ \\
$ \frac{3}{22} \le s < \frac{5}{22} $ & $ \left[11 s - \frac{3}{2}, 1, -11 s + \frac{5}{2}, 11 s - \frac{3}{2}, -11 s + \frac{5}{2}, 11 s - \frac{3}{2}\right] $ & $ w_{5}w_{3}w_{4}w_{2} $ \\
$ \frac{5}{22} \le s < \frac{7}{22} $ & $ \left[1, 1, 11 s - \frac{5}{2}, -11 s + \frac{7}{2}, 11 s - \frac{5}{2}, 1\right] $ & $ w_{4}w_{2} $ \\
$ \frac{7}{22} \le s < \frac{9}{22} $ & $ \left[1, -11 s + \frac{9}{2}, 1, 11 s - \frac{7}{2}, 1, 1\right] $ & $ w_{2} $ \\
$ \frac{9}{22} \le s \le \frac{1}{2} $ & $ \left[1, 11 s - \frac{9}{2}, 1, 1, 1, 1\right] $ & $ 1 $ \\
\end{tabular} \end{table} 
  \end{landscape} \begin{landscape} 
  \begin{table} 
 \caption{$ E _{ 6 }$ Parabolic 3 dom weight} 
 \begin{tabular}{ccc}
Range & dom weight  & w \\
$ 0 \le s < \frac{1}{18} $ & $ \left[9 s + \frac{1}{2}, -9 s + \frac{1}{2}, -9 s + \frac{1}{2}, 18 s, -9 s + \frac{1}{2}, -9 s + \frac{1}{2}\right] $ & $ w_{5}w_{6}w_{3}w_{2}w_{4}w_{5}w_{4}w_{3}w_{2}w_{4}w_{1}w_{3} $ \\
$ \frac{1}{18} \le s < \frac{1}{9} $ & $ \left[1, 9 s - \frac{1}{2}, 9 s - \frac{1}{2}, -18 s + 2, 9 s - \frac{1}{2}, 9 s - \frac{1}{2}\right] $ & $ w_{4}w_{5}w_{3}w_{2}w_{4}w_{1}w_{3} $ \\
$ \frac{1}{9} \le s < \frac{1}{6} $ & $ \left[1, -9 s + \frac{3}{2}, -9 s + \frac{3}{2}, 18 s - 2, -9 s + \frac{3}{2}, 9 s - \frac{1}{2}\right] $ & $ w_{5}w_{3}w_{2}w_{4}w_{1}w_{3} $ \\
$ \frac{1}{6} \le s < \frac{5}{18} $ & $ \left[-9 s + \frac{5}{2}, 9 s - \frac{3}{2}, 9 s - \frac{3}{2}, -9 s + \frac{5}{2}, 9 s - \frac{3}{2}, 1\right] $ & $ w_{4}w_{1}w_{3} $ \\
$ \frac{5}{18} \le s < \frac{7}{18} $ & $ \left[9 s - \frac{5}{2}, 1, -9 s + \frac{7}{2}, 9 s - \frac{5}{2}, 1, 1\right] $ & $ w_{3} $ \\
$ \frac{7}{18} \le s \le \frac{1}{2} $ & $ \left[1, 1, 9 s - \frac{7}{2}, 1, 1, 1\right] $ & $ 1 $ \\
\end{tabular} \end{table} 
  \end{landscape} \begin{landscape} 
  \begin{table} 
 \caption{$ E _{ 6 }$ Parabolic 4 dom weight} 
 \begin{tabular}{ccc}
Range & dom weight  & w \\
$ 0 \le s < \frac{1}{42} $ & $ \left[-7 s + \frac{1}{2}, 14 s, 14 s, -21 s + \frac{1}{2}, 14 s, -7 s + \frac{1}{2}\right] $ & $ w_{4}w_{5}w_{6}w_{1}w_{3}w_{2}w_{4}w_{5}w_{4}w_{1}w_{3}w_{2}w_{4} $ \\
$ \frac{1}{42} \le s < \frac{1}{14} $ & $ \left[-7 s + \frac{1}{2}, -7 s + \frac{1}{2}, -7 s + \frac{1}{2}, 21 s - \frac{1}{2}, -7 s + \frac{1}{2}, -7 s + \frac{1}{2}\right] $ & $ w_{5}w_{6}w_{1}w_{3}w_{2}w_{4}w_{5}w_{4}w_{1}w_{3}w_{2}w_{4} $ \\
$ \frac{1}{14} \le s < \frac{1}{7} $ & $ \left[7 s - \frac{1}{2}, 7 s - \frac{1}{2}, 7 s - \frac{1}{2}, -14 s + 2, 7 s - \frac{1}{2}, 7 s - \frac{1}{2}\right] $ & $ w_{4}w_{5}w_{3}w_{2}w_{4} $ \\
$ \frac{1}{7} \le s < \frac{3}{14} $ & $ \left[7 s - \frac{1}{2}, -7 s + \frac{3}{2}, -7 s + \frac{3}{2}, 14 s - 2, -7 s + \frac{3}{2}, 7 s - \frac{1}{2}\right] $ & $ w_{5}w_{3}w_{2}w_{4} $ \\
$ \frac{3}{14} \le s < \frac{5}{14} $ & $ \left[1, 7 s - \frac{3}{2}, 7 s - \frac{3}{2}, -7 s + \frac{5}{2}, 7 s - \frac{3}{2}, 1\right] $ & $ w_{4} $ \\
$ \frac{5}{14} \le s \le \frac{1}{2} $ & $ \left[1, 1, 1, 7 s - \frac{5}{2}, 1, 1\right] $ & $ 1 $ \\
\end{tabular} \end{table} 
  \end{landscape} \begin{landscape} 
  \begin{table} 
 \caption{$ E _{ 6 }$ Parabolic 5 dom weight} 
 \begin{tabular}{ccc}
Range & dom weight  & w \\
$ 0 \le s < \frac{1}{18} $ & $ \left[-9 s + \frac{1}{2}, -9 s + \frac{1}{2}, -9 s + \frac{1}{2}, 18 s, -9 s + \frac{1}{2}, 9 s + \frac{1}{2}\right] $ & $ w_{1}w_{3}w_{2}w_{4}w_{5}w_{6}w_{4}w_{1}w_{3}w_{2}w_{4}w_{5} $ \\
$ \frac{1}{18} \le s < \frac{1}{9} $ & $ \left[9 s - \frac{1}{2}, 9 s - \frac{1}{2}, 9 s - \frac{1}{2}, -18 s + 2, 9 s - \frac{1}{2}, 1\right] $ & $ w_{4}w_{5}w_{6}w_{3}w_{2}w_{4}w_{5} $ \\
$ \frac{1}{9} \le s < \frac{1}{6} $ & $ \left[9 s - \frac{1}{2}, -9 s + \frac{3}{2}, -9 s + \frac{3}{2}, 18 s - 2, -9 s + \frac{3}{2}, 1\right] $ & $ w_{5}w_{6}w_{3}w_{2}w_{4}w_{5} $ \\
$ \frac{1}{6} \le s < \frac{5}{18} $ & $ \left[1, 9 s - \frac{3}{2}, 9 s - \frac{3}{2}, -9 s + \frac{5}{2}, 9 s - \frac{3}{2}, -9 s + \frac{5}{2}\right] $ & $ w_{6}w_{4}w_{5} $ \\
$ \frac{5}{18} \le s < \frac{7}{18} $ & $ \left[1, 1, 1, 9 s - \frac{5}{2}, -9 s + \frac{7}{2}, 9 s - \frac{5}{2}\right] $ & $ w_{5} $ \\
$ \frac{7}{18} \le s \le \frac{1}{2} $ & $ \left[1, 1, 1, 1, 9 s - \frac{7}{2}, 1\right] $ & $ 1 $ \\
\end{tabular} \end{table} 
  \end{landscape} \begin{landscape} 
  \begin{table} 
 \caption{$ E _{ 6 }$ Parabolic 6 dom weight} 
 \begin{tabular}{ccc}
Range & dom weight  & w \\
$ 0 \le s < \frac{1}{12} $ & $ \left[-12 s + 1, 1, 12 s, -12 s + 1, 12 s, 1\right] $ & $ w_{4}w_{1}w_{3}w_{2}w_{4}w_{5}w_{6} $ \\
$ \frac{1}{12} \le s < \frac{1}{6} $ & $ \left[12 s - 1, -12 s + 2, -12 s + 2, 12 s - 1, 1, 1\right] $ & $ w_{3}w_{2}w_{4}w_{5}w_{6} $ \\
$ \frac{1}{6} \le s < \frac{1}{4} $ & $ \left[1, 12 s - 2, 12 s - 2, -12 s + 3, 1, 1\right] $ & $ w_{4}w_{5}w_{6} $ \\
$ \frac{1}{4} \le s < \frac{1}{3} $ & $ \left[1, 1, 1, 12 s - 3, -12 s + 4, 1\right] $ & $ w_{5}w_{6} $ \\
$ \frac{1}{3} \le s < \frac{5}{12} $ & $ \left[1, 1, 1, 1, 12 s - 4, -12 s + 5\right] $ & $ w_{6} $ \\
$ \frac{5}{12} \le s \le \frac{1}{2} $ & $ \left[1, 1, 1, 1, 1, 12 s - 5\right] $ & $ 1 $ \\
\end{tabular} \end{table} 
  \end{landscape}
