# Supplementary material for: Poles of degenerate Eisenstein series and Siegel-Weil identities for exceptional split groups
Source: arXiv:2205.06288 source file (2022-05-12)
Supplement: Supplementary file 2 [file E7.tex]

\begin{landscape} 
  \begin{table} 
 \caption{$E_{7}$ Parabolic 1 dom weight} 
 \begin{tabular}{ccc}
Range & dom weight  & w \\
$ 0 \le s < \frac{1}{34} $ & $ \left[1, -17 s + \frac{1}{2}, -17 s + \frac{1}{2}, 34 s, -17 s + \frac{1}{2}, 1, 1\right] $ & $ w_{5}w_{6}w_{7}w_{3}w_{2}w_{4}w_{5}w_{6}w_{1}w_{3}w_{4}w_{5}w_{2}w_{4}w_{3}w_{1} $ \\
$ \frac{1}{34} \le s < \frac{3}{34} $ & $ \left[-17 s + \frac{3}{2}, 17 s - \frac{1}{2}, 17 s - \frac{1}{2}, -17 s + \frac{3}{2}, 17 s - \frac{1}{2}, -17 s + \frac{3}{2}, 1\right] $ & $ w_{6}w_{7}w_{4}w_{5}w_{6}w_{1}w_{3}w_{4}w_{5}w_{2}w_{4}w_{3}w_{1} $ \\
$ \frac{3}{34} \le s < \frac{5}{34} $ & $ \left[17 s - \frac{3}{2}, 1, -17 s + \frac{5}{2}, 17 s - \frac{3}{2}, -17 s + \frac{5}{2}, 17 s - \frac{3}{2}, -17 s + \frac{5}{2}\right] $ & $ w_{7}w_{5}w_{6}w_{3}w_{4}w_{5}w_{2}w_{4}w_{3}w_{1} $ \\
$ \frac{5}{34} \le s < \frac{7}{34} $ & $ \left[1, 1, 17 s - \frac{5}{2}, -17 s + \frac{7}{2}, 17 s - \frac{5}{2}, -17 s + \frac{7}{2}, 17 s - \frac{5}{2}\right] $ & $ w_{6}w_{4}w_{5}w_{2}w_{4}w_{3}w_{1} $ \\
$ \frac{7}{34} \le s < \frac{9}{34} $ & $ \left[1, -17 s + \frac{9}{2}, 1, 17 s - \frac{7}{2}, -17 s + \frac{9}{2}, 17 s - \frac{7}{2}, 1\right] $ & $ w_{5}w_{2}w_{4}w_{3}w_{1} $ \\
$ \frac{9}{34} \le s < \frac{11}{34} $ & $ \left[1, 17 s - \frac{9}{2}, 1, -17 s + \frac{11}{2}, 17 s - \frac{9}{2}, 1, 1\right] $ & $ w_{4}w_{3}w_{1} $ \\
$ \frac{11}{34} \le s < \frac{13}{34} $ & $ \left[1, 1, -17 s + \frac{13}{2}, 17 s - \frac{11}{2}, 1, 1, 1\right] $ & $ w_{3}w_{1} $ \\
$ \frac{13}{34} \le s < \frac{15}{34} $ & $ \left[-17 s + \frac{15}{2}, 1, 17 s - \frac{13}{2}, 1, 1, 1, 1\right] $ & $ w_{1} $ \\
$ \frac{15}{34} \le s \le \frac{1}{2} $ & $ \left[17 s - \frac{15}{2}, 1, 1, 1, 1, 1, 1\right] $ & $ 1 $ \\
\end{tabular} \end{table} 
  \end{landscape} \begin{landscape} 
  \begin{table} 
 \caption{$ E _{ 7 }$ Parabolic 2 dom weight} 
 \begin{tabular}{ccc}
Range & dom weight  & w \\
$ 0 \le s < \frac{1}{28} $ & $ \left[14 s, 14 s, 14 s, -28 s + 1, 14 s, -14 s + 1, 14 s\right] $ & $ w_{4}w_{5}w_{6}w_{7}w_{3}w_{2}w_{4}w_{5}w_{6}w_{4}w_{3}w_{2}w_{4}w_{5}w_{1}w_{3}w_{4}w_{2} $ \\
$ \frac{1}{28} \le s < \frac{1}{14} $ & $ \left[14 s, -14 s + 1, -14 s + 1, 28 s - 1, -14 s + 1, -14 s + 1, 14 s\right] $ & $ w_{5}w_{6}w_{7}w_{3}w_{2}w_{4}w_{5}w_{6}w_{4}w_{3}w_{2}w_{4}w_{5}w_{1}w_{3}w_{4}w_{2} $ \\
$ \frac{1}{14} \le s < \frac{3}{28} $ & $ \left[1, 14 s - 1, 14 s - 1, -28 s + 3, 14 s - 1, 14 s - 1, -14 s + 2\right] $ & $ w_{7}w_{4}w_{5}w_{6}w_{3}w_{2}w_{4}w_{5}w_{1}w_{3}w_{4}w_{2} $ \\
$ \frac{3}{28} \le s < \frac{1}{7} $ & $ \left[1, -14 s + 2, -14 s + 2, 28 s - 3, -14 s + 2, 14 s - 1, -14 s + 2\right] $ & $ w_{7}w_{5}w_{6}w_{3}w_{2}w_{4}w_{5}w_{1}w_{3}w_{4}w_{2} $ \\
$ \frac{1}{7} \le s < \frac{3}{14} $ & $ \left[-14 s + 3, 14 s - 2, 14 s - 2, -14 s + 3, 14 s - 2, -14 s + 3, 14 s - 2\right] $ & $ w_{6}w_{4}w_{5}w_{1}w_{3}w_{4}w_{2} $ \\
$ \frac{3}{14} \le s < \frac{2}{7} $ & $ \left[14 s - 3, 1, -14 s + 4, 14 s - 3, -14 s + 4, 14 s - 3, 1\right] $ & $ w_{5}w_{3}w_{4}w_{2} $ \\
$ \frac{2}{7} \le s < \frac{5}{14} $ & $ \left[1, 1, 14 s - 4, -14 s + 5, 14 s - 4, 1, 1\right] $ & $ w_{4}w_{2} $ \\
$ \frac{5}{14} \le s < \frac{3}{7} $ & $ \left[1, -14 s + 6, 1, 14 s - 5, 1, 1, 1\right] $ & $ w_{2} $ \\
$ \frac{3}{7} \le s \le \frac{1}{2} $ & $ \left[1, 14 s - 6, 1, 1, 1, 1, 1\right] $ & $ 1 $ \\
\end{tabular} \end{table} 
  \end{landscape} \begin{landscape} 
  \begin{table} 
 \caption{$ E _{ 7 }$ Parabolic 3 dom weight} 
 \begin{tabular}{ccc}
Range & dom weight  & w \\
$ 0 \le s < \frac{1}{66} $ & $ \left[-11 s + \frac{1}{2}, 22 s, 22 s, -33 s + \frac{1}{2}, 22 s, -11 s + \frac{1}{2}, 1\right] $ & $ w_{4}w_{5}w_{6}w_{7}w_{1}w_{3}w_{2}w_{4}w_{5}w_{6}w_{4}w_{1}w_{3}w_{2}w_{4}w_{5}w_{4}w_{3}w_{2}w_{4}w_{1}w_{3} $ \\
$ \frac{1}{66} \le s < \frac{1}{22} $ & $ \left[-11 s + \frac{1}{2}, -11 s + \frac{1}{2}, -11 s + \frac{1}{2}, 33 s - \frac{1}{2}, -11 s + \frac{1}{2}, -11 s + \frac{1}{2}, 1\right] $ & $ w_{5}w_{6}w_{7}w_{1}w_{3}w_{2}w_{4}w_{5}w_{6}w_{4}w_{1}w_{3}w_{2}w_{4}w_{5}w_{4}w_{3}w_{2}w_{4}w_{1}w_{3} $ \\
$ \frac{1}{22} \le s < \frac{1}{11} $ & $ \left[11 s - \frac{1}{2}, 11 s - \frac{1}{2}, 11 s - \frac{1}{2}, -22 s + 2, 11 s - \frac{1}{2}, 11 s - \frac{1}{2}, -22 s + 2\right] $ & $ w_{7}w_{4}w_{5}w_{6}w_{3}w_{2}w_{4}w_{5}w_{4}w_{3}w_{2}w_{4}w_{1}w_{3} $ \\
$ \frac{1}{11} \le s < \frac{3}{22} $ & $ \left[11 s - \frac{1}{2}, -11 s + \frac{3}{2}, -11 s + \frac{3}{2}, 22 s - 2, -11 s + \frac{3}{2}, -11 s + \frac{3}{2}, 22 s - 2\right] $ & $ w_{5}w_{6}w_{3}w_{2}w_{4}w_{5}w_{4}w_{3}w_{2}w_{4}w_{1}w_{3} $ \\
$ \frac{3}{22} \le s < \frac{2}{11} $ & $ \left[1, 11 s - \frac{3}{2}, 11 s - \frac{3}{2}, -22 s + 4, 11 s - \frac{3}{2}, 11 s - \frac{3}{2}, 1\right] $ & $ w_{4}w_{5}w_{3}w_{2}w_{4}w_{1}w_{3} $ \\
$ \frac{2}{11} \le s < \frac{5}{22} $ & $ \left[1, -11 s + \frac{5}{2}, -11 s + \frac{5}{2}, 22 s - 4, -11 s + \frac{5}{2}, 11 s - \frac{3}{2}, 1\right] $ & $ w_{5}w_{3}w_{2}w_{4}w_{1}w_{3} $ \\
$ \frac{5}{22} \le s < \frac{7}{22} $ & $ \left[-11 s + \frac{7}{2}, 11 s - \frac{5}{2}, 11 s - \frac{5}{2}, -11 s + \frac{7}{2}, 11 s - \frac{5}{2}, 1, 1\right] $ & $ w_{4}w_{1}w_{3} $ \\
$ \frac{7}{22} \le s < \frac{9}{22} $ & $ \left[11 s - \frac{7}{2}, 1, -11 s + \frac{9}{2}, 11 s - \frac{7}{2}, 1, 1, 1\right] $ & $ w_{3} $ \\
$ \frac{9}{22} \le s \le \frac{1}{2} $ & $ \left[1, 1, 11 s - \frac{9}{2}, 1, 1, 1, 1\right] $ & $ 1 $ \\
\end{tabular} \end{table} 
  \end{landscape} \begin{landscape} 
  \begin{table} 
 \caption{$ E _{ 7 }$ Parabolic 4 dom weight} 
 \begin{tabular}{ccc}
Range & dom weight  & w \\
$ 0 \le s < \frac{1}{32} $ & $ \left[8 s, 8 s, 8 s, 8 s, -32 s + 1, 8 s, 8 s\right] $ & $ w_{5}w_{6}w_{7}w_{4}w_{3}w_{2}w_{4}w_{5}w_{6}w_{4}w_{1}w_{3}w_{2}w_{4}w_{5}w_{4}w_{1}w_{3}w_{2}w_{4} $ \\
$ \frac{1}{32} \le s < \frac{1}{24} $ & $ \left[8 s, 8 s, 8 s, -24 s + 1, 32 s - 1, -24 s + 1, 8 s\right] $ & $ w_{6}w_{7}w_{4}w_{3}w_{2}w_{4}w_{5}w_{6}w_{4}w_{1}w_{3}w_{2}w_{4}w_{5}w_{4}w_{1}w_{3}w_{2}w_{4} $ \\
$ \frac{1}{24} \le s < \frac{1}{16} $ & $ \left[8 s, -16 s + 1, -16 s + 1, 24 s - 1, -16 s + 1, 24 s - 1, -16 s + 1\right] $ & $ w_{7}w_{3}w_{2}w_{4}w_{5}w_{6}w_{4}w_{1}w_{3}w_{2}w_{4}w_{5}w_{4}w_{1}w_{3}w_{2}w_{4} $ \\
$ \frac{1}{16} \le s < \frac{1}{12} $ & $ \left[-8 s + 1, 16 s - 1, 16 s - 1, -24 s + 2, 16 s - 1, -8 s + 1, 16 s - 1\right] $ & $ w_{4}w_{5}w_{6}w_{1}w_{3}w_{2}w_{4}w_{5}w_{4}w_{1}w_{3}w_{2}w_{4} $ \\
$ \frac{1}{12} \le s < \frac{1}{8} $ & $ \left[-8 s + 1, -8 s + 1, -8 s + 1, 24 s - 2, -8 s + 1, -8 s + 1, 16 s - 1\right] $ & $ w_{5}w_{6}w_{1}w_{3}w_{2}w_{4}w_{5}w_{4}w_{1}w_{3}w_{2}w_{4} $ \\
$ \frac{1}{8} \le s < \frac{3}{16} $ & $ \left[8 s - 1, 8 s - 1, 8 s - 1, -16 s + 3, 8 s - 1, 8 s - 1, 1\right] $ & $ w_{4}w_{5}w_{3}w_{2}w_{4} $ \\
$ \frac{3}{16} \le s < \frac{1}{4} $ & $ \left[8 s - 1, -8 s + 2, -8 s + 2, 16 s - 3, -8 s + 2, 8 s - 1, 1\right] $ & $ w_{5}w_{3}w_{2}w_{4} $ \\
$ \frac{1}{4} \le s < \frac{3}{8} $ & $ \left[1, 8 s - 2, 8 s - 2, -8 s + 3, 8 s - 2, 1, 1\right] $ & $ w_{4} $ \\
$ \frac{3}{8} \le s \le \frac{1}{2} $ & $ \left[1, 1, 1, 8 s - 3, 1, 1, 1\right] $ & $ 1 $ \\
\end{tabular} \end{table} 
  \end{landscape} \begin{landscape} 
  \begin{table} 
 \caption{$ E _{ 7 }$ Parabolic 5 dom weight} 
 \begin{tabular}{ccc}
Range & dom weight  & w \\
$ 0 \le s < \frac{1}{30} $ & $ \left[10 s, 10 s, 10 s, -30 s + 1, 10 s, 10 s, 10 s\right] $ & $ w_{4}w_{3}w_{2}w_{4}w_{5}w_{6}w_{7}w_{4}w_{1}w_{3}w_{2}w_{4}w_{5}w_{6}w_{4}w_{1}w_{3}w_{2}w_{4}w_{5} $ \\
$ \frac{1}{30} \le s < \frac{1}{20} $ & $ \left[10 s, -20 s + 1, -20 s + 1, 30 s - 1, -20 s + 1, 10 s, 10 s\right] $ & $ w_{3}w_{2}w_{4}w_{5}w_{6}w_{7}w_{4}w_{1}w_{3}w_{2}w_{4}w_{5}w_{6}w_{4}w_{1}w_{3}w_{2}w_{4}w_{5} $ \\
$ \frac{1}{20} \le s < \frac{1}{15} $ & $ \left[-10 s + 1, 20 s - 1, 20 s - 1, -30 s + 2, 20 s - 1, -10 s + 1, 10 s\right] $ & $ w_{4}w_{5}w_{6}w_{7}w_{1}w_{3}w_{2}w_{4}w_{5}w_{6}w_{4}w_{1}w_{3}w_{2}w_{4}w_{5} $ \\
$ \frac{1}{15} \le s < \frac{1}{10} $ & $ \left[-10 s + 1, -10 s + 1, -10 s + 1, 30 s - 2, -10 s + 1, -10 s + 1, 10 s\right] $ & $ w_{5}w_{6}w_{7}w_{1}w_{3}w_{2}w_{4}w_{5}w_{6}w_{4}w_{1}w_{3}w_{2}w_{4}w_{5} $ \\
$ \frac{1}{10} \le s < \frac{3}{20} $ & $ \left[10 s - 1, 10 s - 1, 10 s - 1, -20 s + 3, 10 s - 1, 10 s - 1, -10 s + 2\right] $ & $ w_{7}w_{4}w_{5}w_{6}w_{3}w_{2}w_{4}w_{5} $ \\
$ \frac{3}{20} \le s < \frac{1}{5} $ & $ \left[10 s - 1, -10 s + 2, -10 s + 2, 20 s - 3, -10 s + 2, 10 s - 1, -10 s + 2\right] $ & $ w_{7}w_{5}w_{6}w_{3}w_{2}w_{4}w_{5} $ \\
$ \frac{1}{5} \le s < \frac{3}{10} $ & $ \left[1, 10 s - 2, 10 s - 2, -10 s + 3, 10 s - 2, -10 s + 3, 10 s - 2\right] $ & $ w_{6}w_{4}w_{5} $ \\
$ \frac{3}{10} \le s < \frac{2}{5} $ & $ \left[1, 1, 1, 10 s - 3, -10 s + 4, 10 s - 3, 1\right] $ & $ w_{5} $ \\
$ \frac{2}{5} \le s \le \frac{1}{2} $ & $ \left[1, 1, 1, 1, 10 s - 4, 1, 1\right] $ & $ 1 $ \\
\end{tabular} \end{table} 
  \end{landscape} \begin{landscape} 
  \begin{table} 
 \caption{$ E _{ 7 }$ Parabolic 6 dom weight} 
 \begin{tabular}{ccc}
Range & dom weight  & w \\
$ 0 \le s < \frac{1}{26} $ & $ \left[1, -13 s + \frac{1}{2}, -13 s + \frac{1}{2}, 26 s, -13 s + \frac{1}{2}, -13 s + \frac{1}{2}, 26 s\right] $ & $ w_{6}w_{5}w_{3}w_{4}w_{1}w_{3}w_{2}w_{4}w_{5}w_{6}w_{7}w_{5}w_{3}w_{4}w_{1}w_{3}w_{2}w_{4}w_{5}w_{6} $ \\
$ \frac{1}{26} \le s < \frac{1}{13} $ & $ \left[-13 s + \frac{3}{2}, 13 s - \frac{1}{2}, 13 s - \frac{1}{2}, -26 s + 2, 13 s - \frac{1}{2}, 13 s - \frac{1}{2}, 1\right] $ & $ w_{4}w_{1}w_{3}w_{2}w_{4}w_{5}w_{6}w_{7}w_{4}w_{1}w_{3}w_{2}w_{4}w_{5}w_{6} $ \\
$ \frac{1}{13} \le s < \frac{3}{26} $ & $ \left[-13 s + \frac{3}{2}, -13 s + \frac{3}{2}, -13 s + \frac{3}{2}, 26 s - 2, -13 s + \frac{3}{2}, 13 s - \frac{1}{2}, 1\right] $ & $ w_{1}w_{3}w_{2}w_{4}w_{5}w_{6}w_{7}w_{4}w_{1}w_{3}w_{2}w_{4}w_{5}w_{6} $ \\
$ \frac{3}{26} \le s < \frac{2}{13} $ & $ \left[13 s - \frac{3}{2}, 13 s - \frac{3}{2}, 13 s - \frac{3}{2}, -26 s + 4, 13 s - \frac{3}{2}, 1, 1\right] $ & $ w_{4}w_{5}w_{6}w_{7}w_{3}w_{2}w_{4}w_{5}w_{6} $ \\
$ \frac{2}{13} \le s < \frac{5}{26} $ & $ \left[13 s - \frac{3}{2}, -13 s + \frac{5}{2}, -13 s + \frac{5}{2}, 26 s - 4, -13 s + \frac{5}{2}, 1, 1\right] $ & $ w_{5}w_{6}w_{7}w_{3}w_{2}w_{4}w_{5}w_{6} $ \\
$ \frac{5}{26} \le s < \frac{7}{26} $ & $ \left[1, 13 s - \frac{5}{2}, 13 s - \frac{5}{2}, -13 s + \frac{7}{2}, 13 s - \frac{5}{2}, -13 s + \frac{7}{2}, 1\right] $ & $ w_{6}w_{7}w_{4}w_{5}w_{6} $ \\
$ \frac{7}{26} \le s < \frac{9}{26} $ & $ \left[1, 1, 1, 13 s - \frac{7}{2}, -13 s + \frac{9}{2}, 13 s - \frac{7}{2}, -13 s + \frac{9}{2}\right] $ & $ w_{7}w_{5}w_{6} $ \\
$ \frac{9}{26} \le s < \frac{11}{26} $ & $ \left[1, 1, 1, 1, 13 s - \frac{9}{2}, -13 s + \frac{11}{2}, 13 s - \frac{9}{2}\right] $ & $ w_{6} $ \\
$ \frac{11}{26} \le s \le \frac{1}{2} $ & $ \left[1, 1, 1, 1, 1, 13 s - \frac{11}{2}, 1\right] $ & $ 1 $ \\
\end{tabular} \end{table} 
  \end{landscape} \begin{landscape} 
  \begin{table} 
 \caption{$ E _{ 7 }$ Parabolic 7 dom weight} 
 \begin{tabular}{ccc}
Range & dom weight  & w \\
$ 0 \le s < \frac{1}{18} $ & $ \left[1, 18 s, 1, -18 s + 1, 18 s, -18 s + 1, 18 s\right] $ & $ w_{6}w_{4}w_{5}w_{3}w_{4}w_{1}w_{3}w_{2}w_{4}w_{5}w_{6}w_{7} $ \\
$ \frac{1}{18} \le s < \frac{1}{9} $ & $ \left[1, 1, -18 s + 2, 18 s - 1, -18 s + 2, 18 s - 1, 1\right] $ & $ w_{5}w_{3}w_{4}w_{1}w_{3}w_{2}w_{4}w_{5}w_{6}w_{7} $ \\
$ \frac{1}{9} \le s < \frac{1}{6} $ & $ \left[-18 s + 3, 1, 18 s - 2, -18 s + 3, 18 s - 2, 1, 1\right] $ & $ w_{4}w_{1}w_{3}w_{2}w_{4}w_{5}w_{6}w_{7} $ \\
$ \frac{1}{6} \le s < \frac{2}{9} $ & $ \left[18 s - 3, -18 s + 4, -18 s + 4, 18 s - 3, 1, 1, 1\right] $ & $ w_{3}w_{2}w_{4}w_{5}w_{6}w_{7} $ \\
$ \frac{2}{9} \le s < \frac{5}{18} $ & $ \left[1, 18 s - 4, 18 s - 4, -18 s + 5, 1, 1, 1\right] $ & $ w_{4}w_{5}w_{6}w_{7} $ \\
$ \frac{5}{18} \le s < \frac{1}{3} $ & $ \left[1, 1, 1, 18 s - 5, -18 s + 6, 1, 1\right] $ & $ w_{5}w_{6}w_{7} $ \\
$ \frac{1}{3} \le s < \frac{7}{18} $ & $ \left[1, 1, 1, 1, 18 s - 6, -18 s + 7, 1\right] $ & $ w_{6}w_{7} $ \\
$ \frac{7}{18} \le s < \frac{4}{9} $ & $ \left[1, 1, 1, 1, 1, 18 s - 7, -18 s + 8\right] $ & $ w_{7} $ \\
$ \frac{4}{9} \le s \le \frac{1}{2} $ & $ \left[1, 1, 1, 1, 1, 1, 18 s - 8\right] $ & $ 1 $ \\
\end{tabular} \end{table} 
  \end{landscape}
