# Supplementary material for: Poles of degenerate Eisenstein series and Siegel-Weil identities for exceptional split groups
Source: arXiv:2205.06288 source file (2022-05-12)
Supplement: Supplementary file 3 [file F4.tex]

\begin{landscape} 
  \begin{table} 
 \caption{$F_{4}$ Parabolic 1 dom weight} 
 \begin{tabular}{ccc}
Range & dom weight  & w \\
$ 0 \le s < \frac{1}{16} $ & $ \left[8 s, 8 s, -16 s + 1, 1\right] $ & $ w_{3}w_{4}w_{2}w_{3}w_{2}w_{1} $ \\
$ \frac{1}{16} \le s < \frac{1}{8} $ & $ \left[8 s, -8 s + 1, 16 s - 1, -16 s + 2\right] $ & $ w_{4}w_{2}w_{3}w_{2}w_{1} $ \\
$ \frac{1}{8} \le s < \frac{3}{16} $ & $ \left[1, 8 s - 1, -16 s + 3, 16 s - 2\right] $ & $ w_{3}w_{2}w_{1} $ \\
$ \frac{3}{16} \le s < \frac{1}{4} $ & $ \left[1, -8 s + 2, 16 s - 3, 1\right] $ & $ w_{2}w_{1} $ \\
$ \frac{1}{4} \le s < \frac{3}{8} $ & $ \left[-8 s + 3, 8 s - 2, 1, 1\right] $ & $ w_{1} $ \\
$ \frac{3}{8} \le s \le \frac{1}{2} $ & $ \left[8 s - 3, 1, 1, 1\right] $ & $ 1 $ \\
\end{tabular} \end{table} 
  \end{landscape} \begin{landscape} 
  \begin{table} 
 \caption{$ F _{ 4 }$ Parabolic 2 dom weight} 
 \begin{tabular}{ccc}
Range & dom weight  & w \\
$ 0 \le s < \frac{1}{30} $ & $ \left[10 s, -15 s + \frac{1}{2}, 10 s, 10 s\right] $ & $ w_{2}w_{3}w_{4}w_{1}w_{2}w_{3}w_{1}w_{2} $ \\
$ \frac{1}{30} \le s < \frac{1}{20} $ & $ \left[-5 s + \frac{1}{2}, 15 s - \frac{1}{2}, -20 s + 1, 10 s\right] $ & $ w_{3}w_{4}w_{1}w_{2}w_{3}w_{1}w_{2} $ \\
$ \frac{1}{20} \le s < \frac{1}{10} $ & $ \left[-5 s + \frac{1}{2}, -5 s + \frac{1}{2}, 20 s - 1, -10 s + 1\right] $ & $ w_{4}w_{1}w_{2}w_{3}w_{1}w_{2} $ \\
$ \frac{1}{10} \le s < \frac{1}{5} $ & $ \left[5 s - \frac{1}{2}, 5 s - \frac{1}{2}, -10 s + 2, 10 s - 1\right] $ & $ w_{3}w_{2} $ \\
$ \frac{1}{5} \le s < \frac{3}{10} $ & $ \left[5 s - \frac{1}{2}, -5 s + \frac{3}{2}, 10 s - 2, 1\right] $ & $ w_{2} $ \\
$ \frac{3}{10} \le s \le \frac{1}{2} $ & $ \left[1, 5 s - \frac{3}{2}, 1, 1\right] $ & $ 1 $ \\
\end{tabular} \end{table} 
  \end{landscape} \begin{landscape} 
  \begin{table} 
 \caption{$ F _{ 4 }$ Parabolic 3 dom weight} 
 \begin{tabular}{ccc}
Range & dom weight  & w \\
$ 0 \le s < \frac{1}{42} $ & $ \left[-7 s + \frac{1}{2}, 14 s, -21 s + \frac{1}{2}, 14 s\right] $ & $ w_{3}w_{1}w_{2}w_{3}w_{4}w_{3}w_{1}w_{2}w_{3} $ \\
$ \frac{1}{42} \le s < \frac{1}{14} $ & $ \left[-7 s + \frac{1}{2}, -7 s + \frac{1}{2}, 21 s - \frac{1}{2}, -7 s + \frac{1}{2}\right] $ & $ w_{1}w_{2}w_{3}w_{4}w_{3}w_{1}w_{2}w_{3} $ \\
$ \frac{1}{14} \le s < \frac{1}{7} $ & $ \left[7 s - \frac{1}{2}, 7 s - \frac{1}{2}, -14 s + 2, 7 s - \frac{1}{2}\right] $ & $ w_{3}w_{4}w_{2}w_{3} $ \\
$ \frac{1}{7} \le s < \frac{3}{14} $ & $ \left[7 s - \frac{1}{2}, -7 s + \frac{3}{2}, 14 s - 2, -7 s + \frac{3}{2}\right] $ & $ w_{4}w_{2}w_{3} $ \\
$ \frac{3}{14} \le s < \frac{5}{14} $ & $ \left[1, 7 s - \frac{3}{2}, -7 s + \frac{5}{2}, 7 s - \frac{3}{2}\right] $ & $ w_{3} $ \\
$ \frac{5}{14} \le s \le \frac{1}{2} $ & $ \left[1, 1, 7 s - \frac{5}{2}, 1\right] $ & $ 1 $ \\
\end{tabular} \end{table} 
  \end{landscape} \begin{landscape} 
  \begin{table} 
 \caption{$ F _{ 4 }$ Parabolic 4 dom weight} 
 \begin{tabular}{ccc}
Range & dom weight  & w \\
$ 0 \le s < \frac{1}{22} $ & $ \left[1, -11 s + \frac{1}{2}, 22 s, -11 s + \frac{1}{2}\right] $ & $ w_{4}w_{2}w_{3}w_{1}w_{2}w_{3}w_{4} $ \\
$ \frac{1}{22} \le s < \frac{3}{22} $ & $ \left[-11 s + \frac{3}{2}, 11 s - \frac{1}{2}, -11 s + \frac{3}{2}, 11 s - \frac{1}{2}\right] $ & $ w_{3}w_{1}w_{2}w_{3}w_{4} $ \\
$ \frac{3}{22} \le s < \frac{5}{22} $ & $ \left[11 s - \frac{3}{2}, -11 s + \frac{5}{2}, 11 s - \frac{3}{2}, 1\right] $ & $ w_{2}w_{3}w_{4} $ \\
$ \frac{5}{22} \le s < \frac{7}{22} $ & $ \left[1, 11 s - \frac{5}{2}, -11 s + \frac{7}{2}, 1\right] $ & $ w_{3}w_{4} $ \\
$ \frac{7}{22} \le s < \frac{9}{22} $ & $ \left[1, 1, 11 s - \frac{7}{2}, -11 s + \frac{9}{2}\right] $ & $ w_{4} $ \\
$ \frac{9}{22} \le s \le \frac{1}{2} $ & $ \left[1, 1, 1, 11 s - \frac{9}{2}\right] $ & $ 1 $ \\
\end{tabular} \end{table} 
  \end{landscape}
